# Supplementary material for: The Perfect Victim: Computational Analysis of Judicial Attitudes towards Victims of Sexual Violence
Source: arXiv:2305.05302 source file (2023-05-09)
Supplement: Supplementary file 1 [file 11_appendix_queries.tex]

\appendix
\section{syntactic queries}
\subsection{19 Queries Utilized in Section~\ref{sec:sent_ext}}

\begin{figure}[b]
  \includegraphics[width=8cm,height=10cm,left]{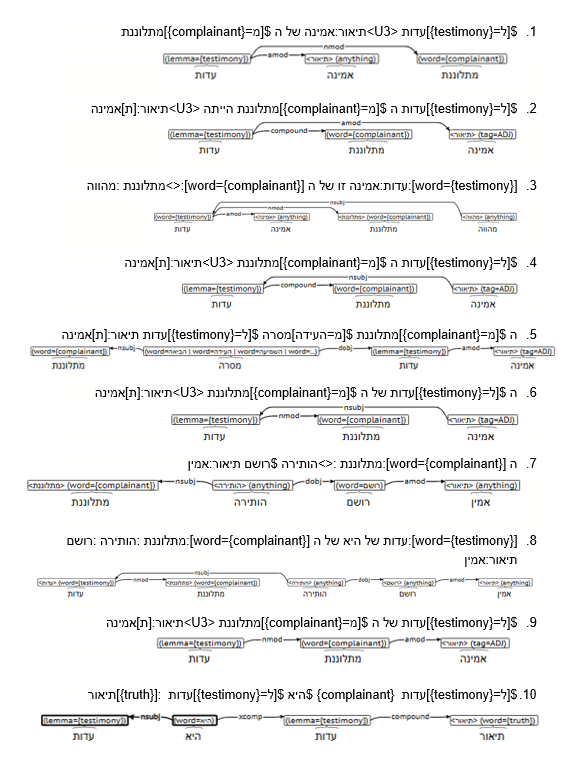}
  \label{figure:q1_tree2}
\end{figure}

\begin{figure}[b]
  \includegraphics[width=8cm,height=10cm,left]{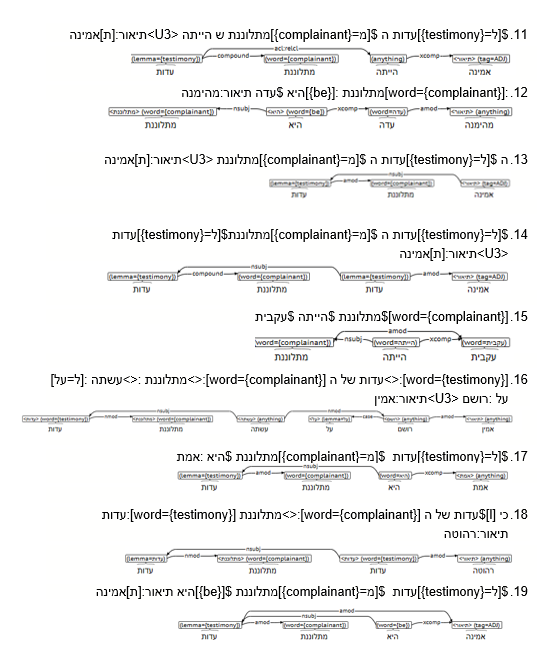}
  \label{figure:q2_tree2}
\end{figure}
